# Supplementary material for: Engineering deterministic, tunable, and reversible folds in graphene with the use of ultrafast laser micro-patterned stretchable polymer substrate
Source: arXiv:2506.18967 source file (2025-06-23)
Supplement: Supplementary file 1 [file JuarezSaborio_ACSnano_SM.pdf]

# SUPPLEMENTARY MATERIALS : Engineering deterministic, tunable, and reversible folds in graphene with the use of ultrafast laser micro-patterned stretchable polymer substrate

A.F. Juarez Saborio,[†,‡] F. Bourquard,[‡] R. Galafassi,[†] A. Claudel,[¶] L. Marty,[¶] A. Piednoir,[†] M. Mercury,[†] R. Fulcrand,[†] C. Albin,[†] V. Barnier,[§] F. Garrelie,[‡] A. San-Miguel,[†] and F. Vialla[*,†]

†*Universite Claude Bernard Lyon 1, ILM Institut Lumiere Matiere, UMR CNRS 5306, 69622 Villeurbanne cedex, FRANCE*

‡*Universite Jean Monnet, Laboratoire Hubert Curien, UMR CNRS 5516, 42000 Saint-Etienne, FRANCE*

¶*Univ. Grenoble Alpes, CNRS, Grenoble INP, Institut Néel, 38000 Grenoble, France*

§*Mines Saint-Etienne, LGF Laboratoire Georges Friedel, UMR CNRS 5307, F-42023 Saint-Étienne cedex 2, FRANCE*

E-mail: fabien.vialla@univ-lyon1.fr

# 1 Traction machine

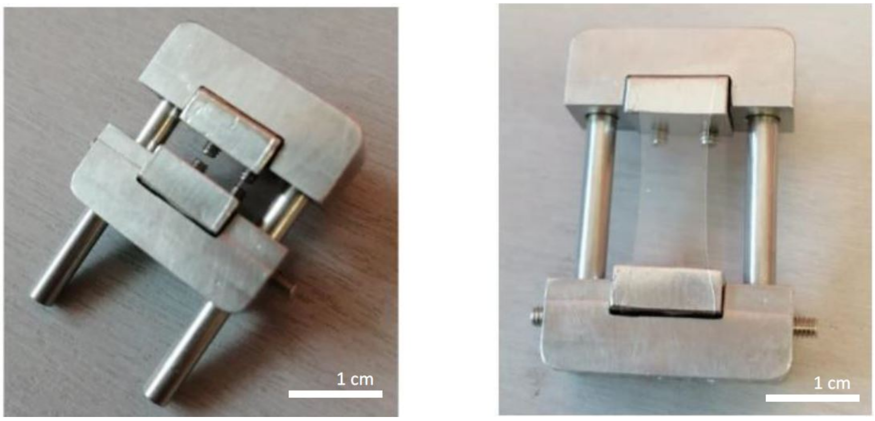


Figure $S1$: Photographs of the PDMS substrate in its unstretched (left) and stretched (right) state within the head of the traction machine. Set of screws allows to fix a given state of stretching during sample characterization. This design allowed *in situ* characterization using AFM and Raman spectroscopy in commercial setups.

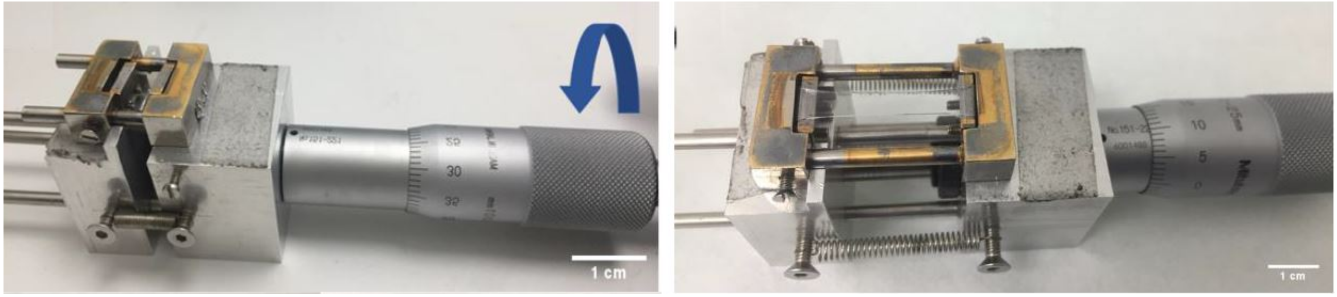


Figure $S2$: Photographs of the traction machine's head integrated into the full device, with an arrow indicating the micrometer screw mechanism used to induce precise control over strain, before (left) and after (right) stretching.

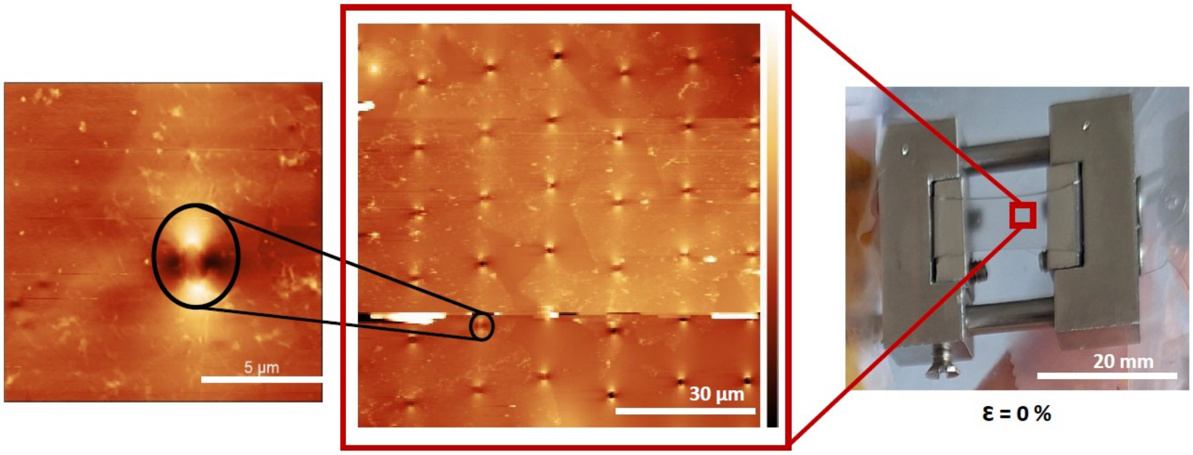


Figure $S3$: Photograph (right), AFM maps at large (center) and small (left) field of view of the graphene on PDMS patterned substrate in its initial state (stretched PDMS and as-transferred uncompressed graphene) in the head of the traction machine.

## 2 Cavity patterning

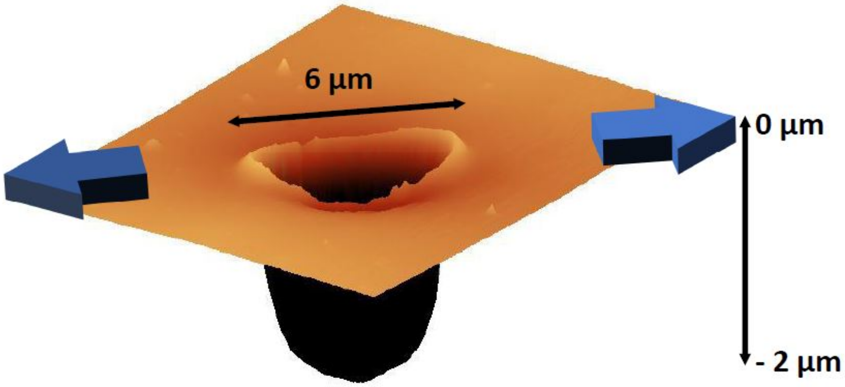


Figure $S4$: 3D representation of AFM data of a textured PDMS cavity prior to graphene deposition, here with a diameter of around 6 $\mu$m (different from the ones presented in the main text). Substrate stretching induces a consistent oval shape elongated along the axis of stretch, with edges rising along this axis and falling in the orthogonal direction, as expected for holes in elastic materials subjected to uniaxial strain. This asymmetric deformation of the cavity may play a crucial role in guiding the subsequent folding behavior of the graphene layer deposited on the substrate (see next section).

# 3 Folding energetics

The observed deterministic nucleation of folds that extend upwards within the cavity contrasts with a behavior of folds that would fall downwards which could be considered more favorable given that the suspended sheet initially penetrates slightly into the cavity. Experimentally, this downward folding behavior has been observed in preliminary samples patterned with linear one-dimensional cavities (trenches). We only and systematically observed upward folds in the case of a zero-dimensional cavity (holes, as presented in this work).

The stable morphology of the graphene sheet is defined by the competition between the energies of stretching, bending, and adhesion.[1] A precise evaluation and prediction of the complex 2D shapes and behaviors presented in this study, as illustrated in main text Fig. 1b, extend beyond the scope of the current investigation. Nonetheless, to elucidate the physical mechanisms leading to fold nucleation, we evaluated the stretching and bending energies along two orthogonal directions — parallel $x$ and perpendicular $y$ to the applied compression — over the suspended region. In this one-dimensional height profile $z(x)$, stretching (related to the strain $\epsilon_G$) and bending (related to the curvature $\kappa_G$) energy densities can be written, respectively:

$$U_S = \frac{1}{2}\,E\,\epsilon_G^2 = \frac{1}{2}\,E\left[1 - \frac{\int\sqrt{dx^2+dz^2}}{L_{0x}}\right]^2$$

$$U_B = \frac{1}{2}\,T\,\kappa_G^2 = \frac{1}{2}\,T\int\left[\frac{\frac{d^2z}{dx^2}}{\left(1+\left(\frac{dz}{dx}\right)^2\right)^{3/2}}\right]^2$$

with $E \sim 1.10^9$ eV/$\mu$m$^2$, $T \sim 1$ eV,[1] and $L_{0x}$ the initial length of suspended graphene. The integrals are evaluated between the two extrema corresponding to the cavity edges. Energy values were evaluated based on ansatz of graphene sheet profiles mimicking the experimental data at low compression ($\epsilon = 1\%$) over a small cavity ($2\mu m$). Both upward ($\Uparrow$) and downward ($\Downarrow$) folding scenarios were considered while assuming clamping of the graphene at the edges. Polynomial functions were introduced, featuring a positive fourth-degree term to represent the overall suspended shape. An additional negative second-degree term is used to account for the upward fold. Upward and downward folding profiles along $x$-

direction are defined with the same length, thus with no relative stretching and only bending variations. We accounted for the Poisson's ratio $\nu = 0.5$ in PDMS for $y$-direction stretching in response to $x$-direction compression. Along the $y$-direction, the matching height at the center of the suspended region with the $x$-direction conditioned the profile parameters. A positive second-degree terms has been added to reduce the length and thus the stretching term along this axis. We find with the profiles presented in Fig. $S5$: $U_{Bx}^{\Uparrow} = 440$ a.u., $U_{Bx}^{\Downarrow} = 290$ a.u., $U_{By}^{\Uparrow} = 100$ a.u., $U_{By}^{\Downarrow} = 50$ a.u., $U_{Sy}^{\Uparrow} = 0$ a.u., $U_{Sy}^{\Downarrow} = 3400$ a.u. Our findings indicate that the bending energy increases more with upward folding compared to downward configuration on the $x$-axis, as expected given the 3 more marked ondulations in the former case compared to the single smoother one in the latter. We also find a slight higher increase in bending energy on the $y$-axis. These would overall indicate a less favorable configuration for the upward fold compared to the downward one. This consideration confirms the experimentally observed downward behaviour in trenches, where the sheet can fall as a whole on the orthogonal $y$-axis. However, in the hole configuration with clamping at the edges considered here, we calculated an increase in stretching energy along the $y$-axis which is significantly higher by more than one order of magnitude in the downward case. This is due to both the Poisson effect (stretching the sheet to the edges) and the matching condition of the central suspended height (stretching the sheet to the bottom). Consequently, to prevent such stretching when falling down the inside the cavity, it appears to be energetically more favorable for the fold to extend upward, which aligns with the observed behavior in our sample.

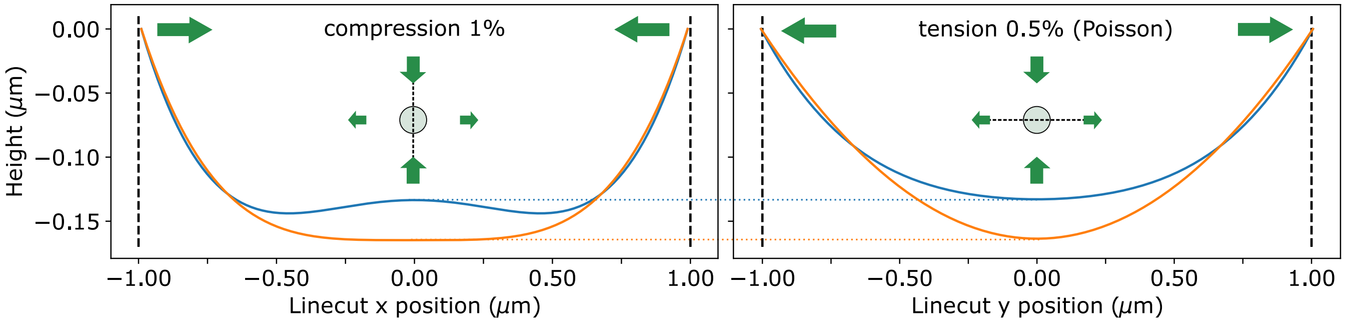


Figure $S5$: Upward ($\Uparrow$, blue) and downward ($\Downarrow$, orange) ansatz profiles of the suspended graphene sheet, for axis parallel ($x$, left) and orthogonal ($y$, right) to the compression direction. Vertical dashed lines at $\pm 1\mu$m mark the cavity edges. Insets illustrate the configuration with the hole cavity at the center, green arrows as compression and Poisson tension vectors, and a dashed line to show the axis of concern in the respective graph.

# 4 Fold profile

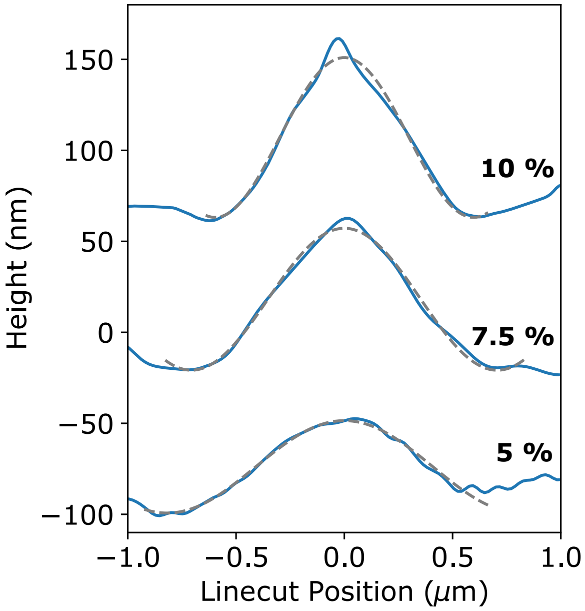


Figure $S6$: Detailed view of the graphene fold formed within the PDMS cavity under applied compression (same data as in main text Fig. 2). The experimental data (blue line) is overlaid with the theoretical cosine profile (grey dashed line). Curves are offset with increasing $\epsilon$ as indicated.

We applied a simple cosine model profile proposed by Vella et al.[2] in their study on delamination of thin films from elastic substrates. The model captures the balance between bending and adhesion energy in the folded system. It has been successfully applied to study stochastic wrinkles in 2D materials.[3] We observe here a good agreement with the overall profile shape. However, the largest deviation from the simple cosine model is found at the highest compression of 10 %. We find a marked point-like fold at the apex of the profile in contrast with the smoother modeled profile. Although thorough study of the graphene folding mechanism falls beyond the current work, we note that our approach yielding deterministic tunable folds enables such a systematic investigation.

# 5 Slipping vs Clamping at cavity edges

We evaluated the suspended length of graphene by analyzing the line cuts from Fig. 2b and 3b, by computing the integral of $\sqrt{dx^2 + dz^2}$ between the two cavity edge maxima, $x$ and $z$ being the profile axis and the height, respectively. The results are presented in Fig. $S7$ as the suspended length of graphene as a function of cavity size with increasing compression. We can define two extreme behaviors: slipping, which occurs when the graphene and cavity share the same trend of size reduction, and clamping, which corresponds to when the length of the graphene is fixed. Our observations reveal a predominance of slipping behavior for the sample depicted in main text Fig. 2 within the explored low compression range ($\epsilon \leq 10\%$). In contrast, the sample illustrated in main text Fig. 3 exhibits an alternation between clamping and slipping behaviors across a larger range of compression. Notably, we observe that the graphene sheet becomes clamped when large compression is reached, and it keeps this behavior over the different steps of the reversible cycle. This observation suggests that a stable clamped behavior over numerous cycles can be reached following an initial stabilizing phase, with interesting potential towards reliable device performances.

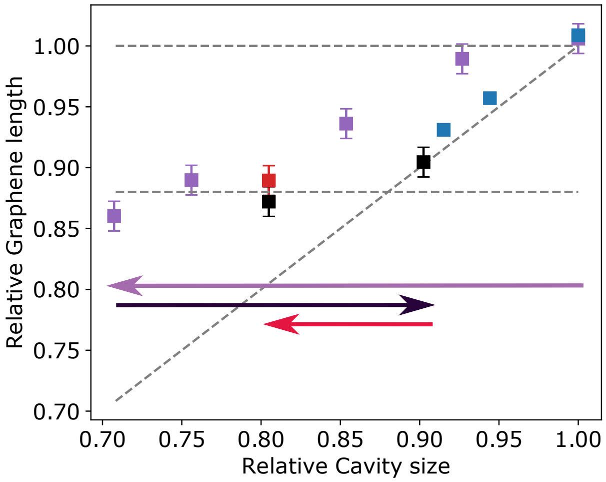


Figure $S7$: Relative change during cycle compression of graphene length ($\int \sqrt{dx^2 + dz^2}$) and cavity size ($\int dx$) between the cavity maxima edges. Square data points correspond to the folding cycle from Fig. 3 with first compression (purple), first release (black), and second compression (red). Horizontal arrows illustrate such cycle. Blue points correspond to data from Fig. 2. Horizontal and diagonal (1:1 slope) grey dashed lines are guide to the eye indicating the clamping and slipping behaviors, respectively. In particular, the horizontal line at relative graphene length of 0.88 indicates a clamped behavior reached at high compression and kept other the cycle.

# 6 Supplementary cavity folds

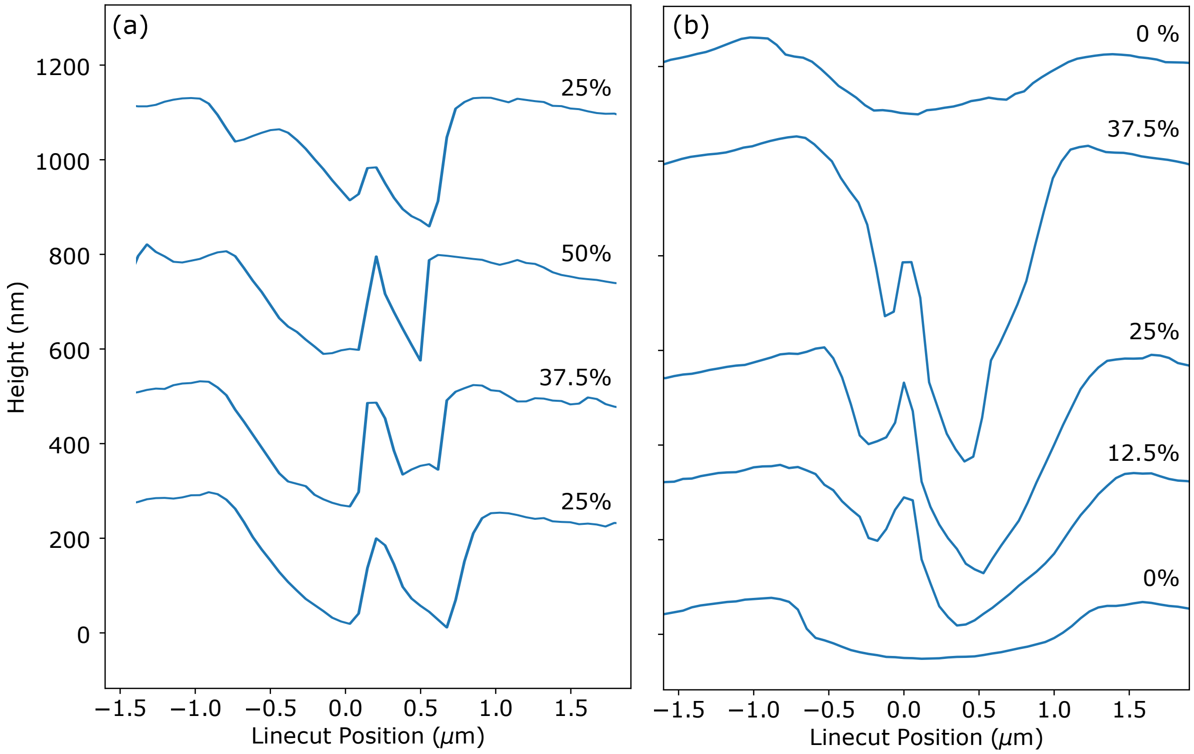


Figure $S8$: (a,b) AFM linecut profiles of graphene suspended over 2 microns wide cavities similarly to the data shown in main text Fig. 3. Compression $\epsilon$ for each curve is indicated, the progressive cycle process being shown from bottom to top.

Looking at alternative folds in Figure $S8$, the general behavior discussed in the main text is preserved, with a deterministic nucleation of a upward fold in the cavity upon compression, and a correlation in height with compression over a cycle process. The consistency of these behaviors across multiple cavities reinforces the robustness of our findings. We however note slightly different elements. In (a), a secondary fold appears to form inside the cavity. In (b), the fold does not nucleate at the center and lowest point of the suspended graphene but rather on the slope of one of the edges. This suggests that nucleation is not simply a cavity geometrical effect but might also be influenced by defects or asymmetries in the graphene sheet prior to compression.

# 7 Supplementary periodic patterns

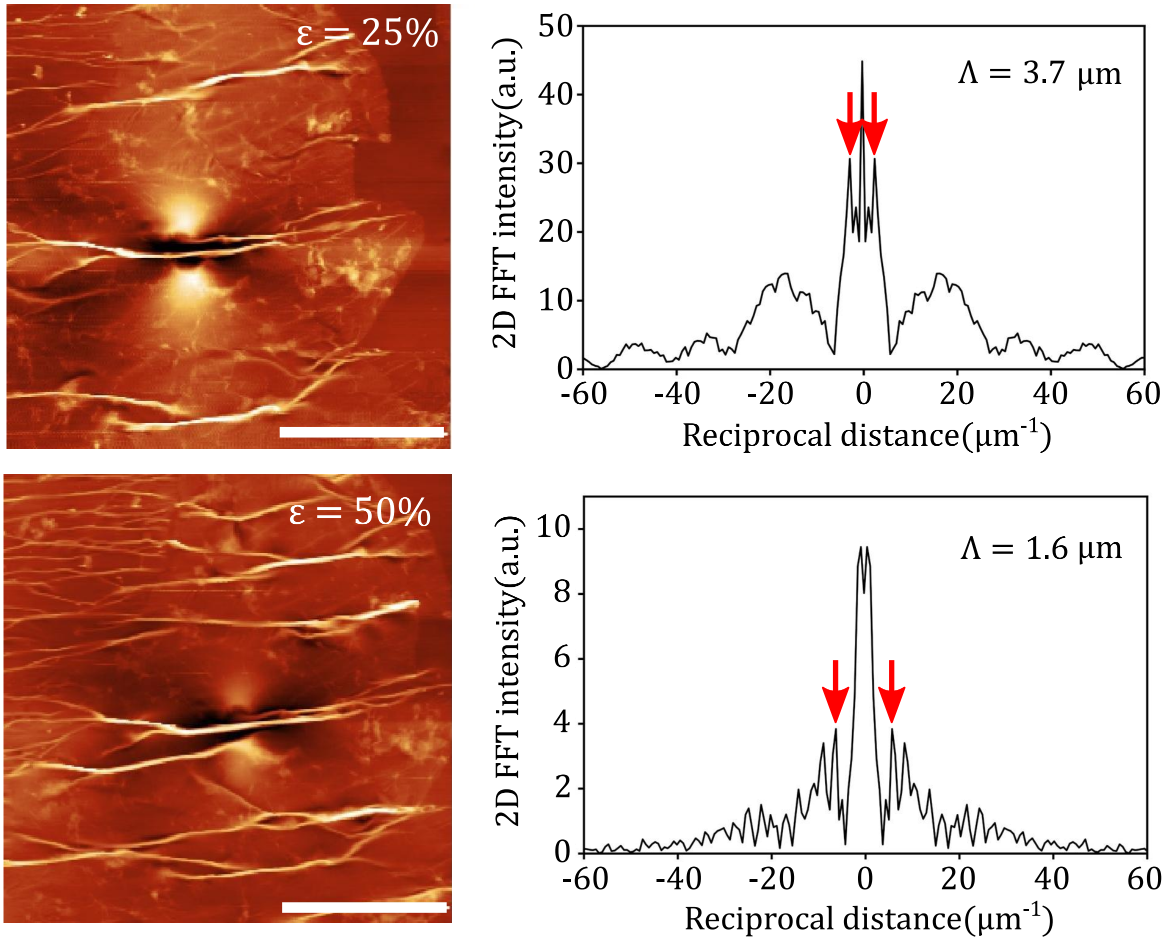


Figure $S9$: AFM map and respective 2D FFT intensity profile along the compression axis for data presented in Figure 3 of the main text, for $\epsilon = 25\%$ (top) and 50% (bottom). Scale bars correspond to 5 $\mu$m. Red arrows indicate the first and main periodicity with a value $\Lambda$ indicated in inset.

The two-dimensional fast Fourier transform (2D-FFT) presented in the main article has also been performed on the AFM data shown in Figure 3. Figure $S9$ shows a clear extracted periodicity with a quantitative value compatible with the one evaluated in Figure 5. Here, evolution from 3.7 to 1.6 $\mu$m (factor 2.3) between the respective compression $\epsilon$ values of 25% to 50% corresponds to the appearance of secondary intermediate folds and the additional not fully transferred macroscopic compression.

# References


(1) Yamamoto, M.; Pierre-Louis, O.; Huang, J.; Fuhrer, M. S.; Einstein, T. L.; Cullen, W. G. "The Princess and the Pea" at the Nanoscale: Wrinkling and Delamination of Graphene on Nanoparticles. *Physical Review X* **2012**, *2*, 041018.

(2) Vella, D.; Bico, J.; Boudaoud, A.; Reis, P. M. The macroscopic delamination of thin films from elastic substrates. *Proceedings of the National Academy of Sciences* **2009**, *106*, 10901–10906.

(3) Brennan, C. J.; Nguyen, J.; Yu, E. T.; Lu, N. Interface Adhesion between 2D Materials and Elastomers Measured by Buckle Delaminations. *Advanced Materials Interfaces* **2015**, *2*, 1500176.
